# Supplementary material for: Multi-Winner Election Control via Social Influence
Source: arXiv:2005.04037 source file (2020-05-28)
Supplement: Supplementary file 1 [file appendix.tex]

\section*{APPENDIX}

\section{Extension of Theorem~\ref{theorem:alphaAppNpHardness} to $t,k>2$}

To generalize the proof for any $k, t > 2$, in constructive model using the general non-increasing scoring function, we set the preferences lists of voters such that the difference between the number of winners from our target party before and after a diffusion is exactly one, if and only if all of the nodes become active.

Consider the minimum $j$ such that $1 \leq i < j \leq |C|$ and $f(i) > f(j)$, i.e., $j$ is the minimum rank that has less score than rank $i = j-1$. 
For example for plurality scoring rule $j=2$, and for anti-plurality $j = |C|$. Note that by assumption there exists such a $j$.
Let us define $a, b$  as $a = f(i), b = f(j)$.

As in the case of $t=3$ and $k=2$, we provide a reduction from the decision version of the deterministic IM problem, to \CMEC and \CDW. 
Let $\mathcal{I}(G, B)$ be an instance for the decision IM problem, where $G = (V, E)$ and $B$, respectively, are the given directed deterministic graph and budget for the IM problem. 
We create an instance $\mathcal{I}'(G', B)$ for the general scoring rule \CMEC and \CDW, where $G'=(V \cup V' \cup V'', E \cup E')$. We consider the same budget, denoted by $B$ for both problems. In order to create $G'$ we do as follows.

\begin{itemize}
    \item For each $v \in V$ we add one more node in $V'$ and it has just one incoming edge from $v$, i.e., $\forall v \in V: v_1 \in V', (v, v_1) \in E'$. By default $V''$ is an empty set.
    
    \item The weight of all edges is 1, i.e., $b_{uv} = 1$ for all $(u, v) \in E \cup E'$.
    
    \item We set the preferences of all nodes $v \in V$ and its new outgoing neighbor as follows:

    \begin{description}
        \item[C1.] If $j \leq k$.
            In this case, for each node $v \in V$ we add $2\alpha$ isolated nodes to the graph where $\alpha = \ceil{\frac{k-1}{i}}$.
            Formally, the graph will be $G' = (V \cup V' \cup V'' , E \cup E')$ where for each node $v \in V$ we have $v_2, v_3, \dots, v_{\alpha+1}, v'_2, v'_3, \dots, v'_{\alpha+1} \in V''$. For simplicity, let us define $k'= k - 1$.
            Also, $V, V', E,$ and $E'$ are defined as before. Note that nodes $v \in V''$ do not have any incoming or outgoing edge. We set the preferences of all nodes as follows. 
            \begin{align*}
                v~ &: \can11 \succ \can21 \dots \succ c_{i-1}^1 \succ \overset{\overset{i}{\downarrow}}{\can12} \succ \overset{\overset{j}{\downarrow}}{\cank1} \succ c_1^3 \succ c_i^1 \succ c_{i+1}^1 \succ \dots \succ c_{k-1}^1 \succ \dots; \\
                v_1 &: \can12 \succ c_i^1 \succ \dots \succ c_{2i-2}^1 \succ \overset{\overset{j}{\downarrow}}{\can13} \succ \overset{\overset{j+1}{\downarrow}}{\cank1} \succ \can11 \succ \dots \succ c_{i-1}^1 \succ c_{2i-1}^1 \succ \\ & \quad \dots \succ c_{k-1}^1 \succ \dots; \\
                v_2 &: \can11 \succ \can21 \succ \dots \succ \overset{\overset{i}{\downarrow}}{c_i^1} \succ \overset{\overset{j}{\downarrow}}{\cank1} \succ \can12 \succ c_j^1 \succ \dots \succ c_{k-1}^1 \succ \dots ;\\
                v'_2 &: \can11 \succ \can21 \succ \dots \succ \overset{\overset{i}{\downarrow}}{c_i^1} \succ \overset{\overset{j}{\downarrow}}{\can12} \succ \cank1 \succ c_j^1 \succ \dots \succ c_{k-1}^1 \succ \dots ;\\
                v_3 &: c_{i\%k' + 1}^1 \succ c_{(i+1)\%k' +1}^1 \succ \dots \succ \overset{\overset{i}{\downarrow}}{c_{(2i-1)\%k'+1}^1} \succ \overset{\overset{j}{\downarrow}}{\cank1} \succ \\ & \quad \can12 \succ c_{(2i)\%k'+1}^1 \succ \dots \succ c_{(i+k'-1)\%k'+1}^1 \succ \dots ;\\
                v'_3 &: c_{i\%k' + 1}^1 \succ c_{(i+1)\%k' +1}^1 \succ \dots \succ \overset{\overset{i}{\downarrow}}{c_{(2i-1)\%k'+1}^1} \succ \overset{\overset{j}{\downarrow}}{\can12} \succ \\ & \quad \cank1 \succ c_{(2i)\%k'+1}^1 \succ \dots \succ c_{(i+k'-1)\%k'+1}^1 \succ \dots;\\
                v_4 &: c_{2i\%k' + 1}^1 \succ c_{(2i+1)\%k' +1}^1 \succ \dots \succ \overset{\overset{i}{\downarrow}}{c_{(3i-1)\%k'+1}^1} \succ \overset{\overset{j}{\downarrow}}{\cank1} \succ \\ & \quad \can12 \succ c_{(3i)\%k'+1}^1 \succ \dots \succ c_{(2i+k'-1)\%k'+1}^1 \succ \dots;\\
                v'_4 &: c_{2i\%k' + 1}^1 \succ c_{(2i+1)\%k' +1}^1 \succ \dots \succ \overset{\overset{i}{\downarrow}}{c_{(3i-1)\%k'+1}^1} \succ \overset{\overset{j}{\downarrow}}{\can12} \succ \\ & \quad \cank1 \succ c_{(3i)\%k'+1}^1 \succ \dots \succ c_{(2i+k'-1)\%k'+1}^1 \succ \dots ;\\
                \vdots\\
                v_{\alpha+1} &: c_{((\alpha-1) i)\%k'+1}^1 \succ c_{((\alpha-1) i+1 )\% k' + 1}^1                 \succ \dots \succ  \overset{\overset{i}{\downarrow}}{c_{(\alpha i - 1) \% k' +1}^1} \succ \overset{\overset{j}{\downarrow}}{\cank1} \succ \\ & \quad \can12 \succ c_{(\alpha i) \% k' +1}^1 \succ \dots \succ
                c_{((\alpha-1) i + k' -1) \% k' +1}^1 \succ \dots;\\
                v'_{\alpha+1} &: c_{((\alpha-1) i)\%k'+1}^1 \succ c_{((\alpha-1) i+1 )\% k' + 1}^1 \succ \dots \succ  \overset{\overset{i}{\downarrow}}{c_{(\alpha i - 1) \% k' +1}^1} \succ \overset{\overset{j}{\downarrow}}{\can12} \succ \\ & \quad \cank1 \succ c_{(\alpha i) \% k' +1}^1 \succ \dots \succ c_{((\alpha-1) i + k' -1) \% k' +1}^1 \succ \dots.
            \end{align*}
            
            In this case, for $1 \leq i \leq k-1$ all the candidates $c_i \in C_1, \can12 \in C_2$ have more votes than $\cank1$; also, every other candidates has at most the same score of $\cank1$. Hence, $\F(C_1, \emptyset) = k-1, \F(C_2, \emptyset) = 1$, for all $3 \leq j \leq t, \F(C_j, \emptyset) = 0$.

        \item[C2.] If $k < j < |C|$.
            \begin{align*}
                v~ &: \can11 \succ \dots \succ c_{k-1}^1 \succ \can22 \succ \dots \succ \cank2 \succ \can13 \succ \dots \succ \overset{\overset{i}{\downarrow}}{\can12} \succ \overset{\overset{j}{\downarrow}}{\cank1} \succ \dots; \\
                v_1 &: \can11 \succ \can21 \succ \dots \succ c_{k-1}^1 \succ \can22 \succ \dots \succ \cank2 \succ \dots \succ \overset{\overset{j}{\downarrow}}{\can13} \succ \overset{\overset{j + 1}{\downarrow}}{\cank1} \succ \dots.
            \end{align*}
        Also in this case, for $1 \leq i \leq k-1$ all the candidates $c_i \in C_1, \can12 \in C_2$ have more votes than $\cank1$; and every other candidates has at most the same score of $\cank1$. Hence, $\F(C_1, \emptyset) = k-1, \F(C_2, \emptyset) = 1$, for all $3 \leq j \leq t, \F(C_j, \emptyset) = 0$.

        \item[C3.] If $j = |C|$. In this case, we add an extra candidate called $c_{1}^{t+1}$ to the candidates ($C = C \cup \{c_1^{t+1} \}$), and then we set the preferences list as follows:

        \begin{align*}
            v~ &: \can11 \succ \dots \succ c_{k-1}^1 \succ \can22 \succ \dots \succ \cank2 \succ \can13 \succ \dots \succ \overset{\overset{i}{\downarrow}}{\can12} \succ \overset{\overset{j}{\downarrow}}{\cank1} \succ c_1^{t+1}; \\
            v_1 &: \can11 \succ \can21 \succ \dots \succ c_{k-1}^1 \succ \can12 \succ \dots \succ \cank2 \succ \dots \succ  \overset{\overset{j}{\downarrow}}{c_1^{t+1}} \succ \overset{\overset{j + 1}{\downarrow}}{\cank1}.
        \end{align*}
        The extra candidate will not be among winners before and after any diffusion. 
        We just add it to the candidates to be able to put the candidate $\cank1 \in C_1$ in position $j+1$.
    \end{description}
\end{itemize}

By this reduction, before any diffusion, in all cases, $k-1$ winner will be from our target part $C_1$, and one winner from party $C_2$.

In $\mathcal{I}'(G', B)$, concerning all cases, all of the nodes $v \in V \cup V'$ become active if and only if all of the nodes $v \in V$ become active. Indeed, by definition, if $V \subseteq A_S$, then for each node $u \in V'$ there exists an incoming neighbor $v \in V$ s.t. $(v, u) \in E'$ and $b_{vu} = 1$, then if $v$ is active, also $u$ becomes active.

Suppose there exists an $\alpha-$approximation algorithm called \textit{$\alpha$-appAlg} for \CDW (respectively, \CMEC) and it returns $S \subseteq V \cup V' \cup V''$ as a solution. 
We show that, by using the seed nodes $S$ returned by the algorithm \textit{$\alpha$-appAlg}, we can find the answer for the decision IM problem.
We will show that $\DOW(C_1, S) > 0$ (resp. $\MOV(C_1, S) > 0$) if and only if $S$ activates all of the nodes in $V \cup V'$, i.e.,  $A_S = V \cup V'$, where  $A_S$ is the set of activated nodes after $S$. That is, since $G$ is a subgraph of $(V \cup V', E \cup E')$, then  $\DOW(C_1, S) > 0$ (respectively, $\MOV(C_1, S) > 0$) if and only if the answer to the decision IM problem is YES.

In order to show if $\DOW(C_1, S) > 0$ (resp. $\MOV(C_1, S) > 0$), then $S$ activates all of the nodes in $V \cup V'$, i.e.,  $V \cup V' \subseteq A_S$, first we show that by $S' \subset V \cup V' \cup V''$ returned by \textit{$\alpha$-appAlg}, we can find a new seed nodes $S \subseteq V$ s.t. $\DOW(C_1, S') = \DOW(C_1, S)$ (also $\MOV(C_1, S') = \MOV(C_1, S)$). 
We construct $S$ as follows:
\begin{itemize}
    \item All of the nodes $u \in S' \cap V$ will be in the $S$ as well.
    
    \item For all of the nodes $u \in S' \cap V'$, we replace them with their single incoming neighbor, i.e., we replace $u$ with the node $v \in V$ s.t. $(v, u) \in E'$. In this case, the target candidate will get at least the same score as before.
    
    \item If the algorithm selects a node $v \in V''$ (in case \textbf{C1}), for all of the nodes $u \in S' \cap V''$, if there exists an isolated node $v \in V \setminus S'$, we replace $u$ with $v$ in the $S$, i.e., we replace $u$ with an arbitrary node in $\{w~|~w \in V \setminus S', \forall v' \in V: (v', w) \notin E \land (w, v') \notin E \}$; if the set is empty, then we replace $u$ with an arbitrary node in $ \{w ~|~ w \in V \setminus S' \}$; since $B \leq |V|$, then the set cannot be empty.
    In the following, we show that by using this substitution, we will get the same value for both $\DOW(C_1, S')$ and $\DOW(C_1, S)$. Let us consider the following cases:

    \begin{itemize}
        \item The algorithm selected $u$ while there exists an isolated node $v \in V$, i.e., there exists a node $v \in V \setminus S'$ which does not have any incoming or outgoing neighbor in $V$; in this case, we replace $u$ with $v$ in the seed nodes $S$, and the target candidate gets the same score as before. Then $\DOW(C_1, S') \leq \DOW(C_1, S)$ (also $\MOV(C_1, S') \leq \MOV(C_1, S)$).
        
        \item The algorithm selected $u \in V''$ as a seed node in $S'$, because all of the nodes $v \in V \cup V'$ will be activated by the seed nodes $S'' = S' \setminus \{u\}$. 
        In this case, since it is enough to activate all nodes of $V \cup V'$ to get the maximum value for \DOW (resp. \MOV), then if we even remove the node $u$ from the seed nodes, it still will activate all nodes of $V \cup V'$, and $\DOW(C_1, S') = \DOW(C_1, S)$ (resp. $\MOV(C_1, S') = \MOV(C_1, S)$).
        By the way, we replace $u$ with $v \in V \setminus S'$ in the seed nodes $S$, but $\DOW(C_1, S)$ will be the same as $\DOW(C_1, S')$; because in this case, $\DOW(C_1, S')$ has the maximum value by activating all nodes $v \in V \cup V'$, and $S$ activates them too; then $\DOW(C_1, S) = \DOW(C_1, S')$.
        In other words, if the algorithm can activate all of the nodes $v \in V$ then all of the target candidates will win the election. 
    \end{itemize}
    Note that it is not possible to have a node $u \in V'' \cup S'$ and a node $v \in V \setminus A_{S'}$ where $v$ is not isolated, at the same time;
    because, if there exists such a node $v$, \textit{$\alpha$-appAlg} could replace $u$ with $v$ (or the incoming neighbor of $v$) and increases the score of its target candidate with the same budget.
    
\end{itemize}

Then, from now on, we assume that \textit{$\alpha$-appAlg} returns the seed nodes $S$, s.t. $S \in V$.
Now we show that if $\DOW(C_1, S) > 0$ (resp. $\MOV(C_1, S) > 0$), then $S$ activates all of the nodes in $V \cup V'$, i.e.,  $A_S = V \cup V'$. 
By contradiction, assume $S$ is a solution for the problem s.t. $\DOW(C_1, S) > 0$ (resp. $\MOV(C_1, S) > 0$), and $S$ does not activate all nodes of $V \cup V'$, i.e., there exists a node $v$ s.t. $v \in V \setminus A_S$.
In this case, for the score of candidates, for all cases,  according to the preferences lists, the candidate $\can11$ will have at least $a-b$ score less than candidates  $\can21, \dots, \cank1, \can12$, which means $\F(C_1, S) = k-1$. According to the definition of $\DOW$ we have $\DOW(C_1, S) = 0$ (also, $\MOV(C_1, S) = 0$), which is a contradiction.
On the other hand, to show that if $S$ activates all the nodes $V \cup V'$, then $\DOW(C_1, S) > 0$ (resp. $\MOV(C_1, S) > 0$), note that if all nodes $V \cup V'$ become active, the score of all candidates $c \in C_1$ will be more than or equal to all other candidates. 
Then by using the tie breaking rule, $\F(C_1, S) = k$, and $2 \leq n \leq t: \F(C_n, S) = 0$, which yields $\DOW(C_1, S) > 0$ (resp. $\MOV(C_1, S) > 0$).
Then, on one side, if $S$ is an answer to the \DMEC or \DDW, it activates all $2n$ nodes in $V \cup V'$.
On the other side, since $G$ is subgraph of $(V \cup V', E \cup E')$, and $S \subseteq V$, then $S$ activates all nodes in $G$.

%=============================================
%=============================================

\section{Extension of Theorem~\ref{theorem:SPVNPHardness} to $t,k>2$}

In this section, we generalize the proof for any $k, t > 2$, regarding the constructive model and general non-increasing scoring function.
The idea is the same as before, and we need to set the preferences list of the voters such that at least one of the candidates changes the score of the target party $C_1$ if the node becomes active. For example, assume the scoring function is plurality, and we set the preferences lists of all nodes as $\can12 \succ \can22 \succ \dots$. Then score of $C_1$ will be the same, before and after any diffusion; hence we cannot distinguish between them. But, if we set the preferences list as $\can12 \succ \can11 \succ \dots$, the score of $C_1$ before and after a diffusion process will change as much as the number of activated nodes after the process.

The same as before, we consider the $i, j$ with the same definition, i.e., the minimum $j$ such that $1 \leq i < j \leq |C|$ and $f(i) > f(j)$, i.e., $j$ is the minimum rank that has less score than rank $i = j-1, 2 \leq j \leq |C| = tk$. For simplicity, Let us define $a = f(i), b = f(j)$.
Also, we reduce the decision and deterministic version of IM problem to $\MOV$ and $\DOV$. 
Assume $\mathcal{I}(G, B)$ is an instance for the decision IM problem, where $G = (V, E)$ and $B$ are the given directed deterministic graph and budget, respectively. 
We create $\mathcal{I}'(G', B)$ as an instance for $\MOV$ and $\DOV$, where $G'=G$, and the same budget, denoted by $B$, for both problems. To create the preferences list of the nodes in $G'$ we do as follows.

\begin{description}
    \item[C1.] If $j \leq k$. $v: \can12  \succ \can22 \succ \dots \succ \overset{\overset{i}{\downarrow}}{c_i^2} \succ \overset{\overset{j}{\downarrow}}{\can11} \succ \can21 \succ \dots \succ \cank1 \succ c_j^2 \succ \dots$. In this case, %score of the party $C_1$ before any diffusion is    
    $\F_{\SPVF}(C_1, \emptyset) = |V|\sum_{j \leq l < j+k} f(l)$.

    \item[C2.] If $j > k$. $v: \can11 \succ \can21 \succ \dots \succ c_{k-1}^1 \succ \can12 \succ \can22 \succ \dots \succ \overset{\overset{j}{\downarrow}}{\cank1} \succ \dots $. In this case, %score of the party $C_1$ before any diffusion is
    $\F_{\SPVF}(C_1, \emptyset) = (a(k-1) + b)|V|$.
\end{description}
By this preferences assignment, if all of the nodes become active after $S$, then $\F_{\SPVF}$ and $\DOV^{\SPVF}$ for party $C_1$ will be as following.
\begin{description}
    \item[C1.] $\F_{\SPVF}(C_1, S) = |V|\sum_{i \leq l < i+k} f(l),$
    \begin{align*}
        \DOV^{\SPVF}(C_1, S) 
        &= |V|\sum_{i \leq l < i+k} f(l) - |V|\sum_{j \leq l < j+k} f(l) \\
        &= (f(i) - f(i+k))|V|;
    \end{align*}
    and, if at least one node is not active $\DOV^{\SPVF}(C_1, S) < (f(i) - f(i+k))|V|$.

    \item[C2.] $\F_{\SPVF}(C_1, S) = ak|V|,$
    \begin{align*}
        \DOV^{\SPVF}(C_1, S)
        &= ak|V| - (a(k-1) + b)|V| \\
        &= (a - b)|V|;
    \end{align*}
    also, if at least one node is not active $\DOV^{\SPVF}(C_1, S) < (a - b)|V|$.
\end{description}
Then by this reduction, we can distinguish between the case that all of the nodes become active or not, which is the answer of IM problem.
Regarding $\MOV^{\SPVF}$, if all of the nodes $v \in V$ become active we have:
\begin{description}
    \item[C1.] In this case, the party with the most score before and after any diffusion process is $C_2$. Then if all of the nodes become active after a diffusion, the score of $C_2$ will reduce by $(f(i) - f(i+k))|V|$.
    In other words, whatever $C_2$ loses will add to $C_1$; then $\MOV^{\SPVF}(C_1, S) = 2\DOV^{\SPVF}(C_1, S)$.

    \item[C2.] In this case, we have two different situations as follows.
    \begin{description}
        \item[C2.1.] If $j \leq 2k$; then the party with most score before and after any diffusion is $C_2$. Similar to case \textbf{C1}, $\MOV^{\SPVF}(C_1, S) = 2\DOV^{\SPVF}(C_1, S)$.
        
        \item[C2.2.] If $2k < j$; the party with the most score before and after $S$ is still $C_2$, but the score of $C_2$ will not reduce after any diffusion, i.e., 
        $\MOV^{\SPVF}(C_1, S) = \F_{\SPVF}(C_1, S) - \F_{\SPVF}(\Cmoa{S}, S) - \left( \F_{\SPVF}(C_1, \emptyset) - \F_{\SPVF}(\Cmob, \emptyset) \right)
        = ak|V| - ak|V| - \Big((a(k-1) + b)|V|) - ak|V| \Big) = (a - b)|V|.$
        
        % \item[C2.3.] if $j \geq 3k$; the party with most score can be any of other $k-2$ parties including $C_2$. Then this case will be same as \textbf{C2.2}.
    \end{description}
\end{description}

Note that if there exists at least one inactive node in $G'$ after $S$, then the value of $\MOV^{\SPVF}(C_1, S)$ will be less than what is determined above. By this, we can understand if all of the nodes can be activated by a set of seed nodes $S$, which is the answer of IM problem.

To present a reduction from the deterministic and decision version of IM problem to $\DOVD$ and $\MOVD$, it is very similar to the constructive model. Except that we should set the preferences list of the nodes $v \in V$ such that at least one of the candidates $c \in C_1$ can decrease the score of $C_1$. The same approach proves the $\NP$-hardness of destructive model too. 

%=============================================
%=============================================

\section{Hardness of approximation for \SPV}
\begin{theorem}
It is $\NP$-hard to approximate the $\MOV^{\SPVF}$ and $\DOV^{\SPVF}$ to within better than a factor $1-\frac{1}{e}$.
\end{theorem}

\begin{proof}
Consider an instance of IM problem $\I(G, B)$ using Independent Cascade (IC) model. 
We reduce it to an instance of \SPV problem $\I'(G, B)$, using the same graph $G = (V, E)$, and budget $B$ for both problems.
We define $i, j$ the same as before, i.e., the minimum $j$ such that $1 \leq i < j \leq |C|$ and $f(i) > f(j)$, i.e., $j$ is the minimum rank that has less score than rank $i = j-1, 2 \leq j \leq |C| = tk$. 
For simplicity, we set $a = f(i), b = f(j)$.
Also, we set the preferences list of each node $v \in V$ as follows.
\begin{description}
    \item[C1.] If $j \leq k$. $v: \can12  \succ \can22 \succ \dots \succ \overset{\overset{i}{\downarrow}}{c_i^2} \succ \overset{\overset{j}{\downarrow}}{\can11} \succ \can21 \succ \dots \succ \cank1 \succ c_j^2 \succ \dots$. In this case,  
    $\F_{\SPVF}(C_1, \emptyset) = |V|\sum_{l = j}^{j+k-1} f(l)$.

    \item[C2.] If $j > k$. $v: \can11 \succ \can21 \succ \dots \succ c_{k-1}^1 \succ \can12 \succ \can22 \succ \dots \succ \overset{\overset{j}{\downarrow}}{\cank1} \succ \dots $. In this case,
    $\F_{\SPVF}(C_1, \emptyset) = (a(k-1) + b)|V|$.
\end{description}

Assume $S$ is the set of seed nodes selected for IM, and $A_S$ is the set of activated nodes after $S$. If we use the same seed set to maximize $\DOV^{\SPVF}$ problem, we have:
\begin{description}
    \item[C1.]
    \begin{align*}
        \F_{\SPVF}(C_1, S) &= |A_S|\sum_{l = i}^{i+k-1} f(l) + |V \setminus A_S|\sum_{l = j}^{j+k-1} f(l) \\
        \DOV^{\SPVF}(C_1, S) &= |A_S|\sum_{l = i}^{i+k-1} f(l) + |V \setminus A_S|\sum_{l = j}^{j+k-1} f(l) - |V|\sum_{l = j}^{j+k-1} f(l) \\
        &= |A_S|\Big(f(i) - f(i+k) \Big)
    \end{align*}
    
    \item[C2.] 
    \begin{align*}
        \F_{\SPVF}(C_1, S) &= ak|A_S| + |V \setminus A_S|\Big(a(k-1) + b\Big)\\
        \DOV^{\SPVF}(C_1, S) &= ak|A_S| + |V \setminus A_S|\Big(a(k-1) + b\Big) - \Big(a(k-1) + b\Big)|V|\\
        &= |A_S|(a - b)
    \end{align*}
\end{description}

On the other hand, if $S$ is the set of seeds to maximize $\DOV^{\SPVF}$, and $A_S$ is the set of active nodes after $S$, and we use the same seed set for IM problem, then we can activate $|A_S|$ nodes if 
\begin{description}
    \item[C1.] 
    \begin{align}
    \label{C1:dov}
        \DOV^{\SPVF}(C_1, S) = |A_S|\Big(f(i) - f(i+k) \Big)
    \end{align}
    \item[C2.] 
    \begin{align}
    \label{C2:dov}
        \DOV^{\SPVF}(C_1, S) = |A_S|(a - b)
    \end{align}
\end{description}

Overall, we prove that $|A_S|$ nodes will be activated by seed set $S$ if and only if using $S$ for maximizing $\DOV^{\SPVF}$, we get~\eqref{C1:dov} or~\eqref{C2:dov}. 
Since it is hard to approximate IM problem better than $1-\frac{1}{e}$ then it yields the same hardness of approximation for maximizing $\DOV^{\SPVF}$.

%\todo{MAM: I have to finalize this part.}
Using the same reduction, we can prove the hardness of approximation for $\MOV^{\SPVF}$.
To see that, note that if we have seed set $S$ and $A_S$ are the activated nodes after $S$, then 
\begin{description}
    \item[C1.] In this case, party $C_2$ is the most scored opponent before and after $S$; then it yields
    \begin{align*}
        &\MOV^{\SPVF}(C_1, S) = \F_{\SPVF}(C_1, S) - \F_{\SPVF}(C_2, S) - \Big( \F_{\SPVF}(C_1, \emptyset) - \F_{\SPVF}(C_2, \emptyset) \Big)\\
        &= |A_S|\sum_{l = i}^{i+k-1} f(l) + |V \setminus A_S|\sum_{l = j}^{j+k-1} f(l) - |V| \Big(\sum_{l=1}^{l = i-1}f(l) + \sum_{l = i+k}^{2k} f(l)\Big) - \\ & \quad \Big(|V|\sum_{l = j}^{j+k-1} f(l) - |V| (\sum_{l=1}^{l = i}f(l) + \sum_{l = j+k}^{2k} f(l)) \Big) \\
        & = |V|\Big(f(i) - f(i+k)\Big) + |A_S|\Big(f(i) - f(i+k)\Big)
    \end{align*}
    Note that in this case, since the party with the most scored before and after $S$ is $C_2$, then whatever $C_2$ loses, our target party $C_1$ will gain, and the score of other parties is the same as before diffusion. Then $\MOV^{\SPVF}(C_1, S) = 2\DOV^{\SPVF}(C_1, S)$.
    
    \item[C2.] In this case, we have two different situations:
    \begin{description}
        \item[C2.1.] If $j \leq 2k$; then the party with most score before and after any diffusion is $C_2$. Similar to case \textbf{C1}, $\MOV^{\SPVF}(C_1, S) = 2\DOV^{\SPVF}(C_1, S)$.
        
        \item[C2.2.] If $2k < j$; the party with the most score before and after $S$ is still $C_2$, but the score of $C_2$ will not reduce after any diffusion, i.e., 
        $\MOV^{\SPVF}(C_1, S) = \F_{\SPVF}(C_1, S) - \F_{\SPVF}(\Cmoa{S}, S) - \left( \F_{\SPVF}(C_1, \emptyset) - \F_{\SPVF}(\Cmob, \emptyset) \right)
        = ak|V| - ak|V| - \Big((a(k-1) + b)|V|) - ak|V| \Big) = (a - b)|V|.$
    \end{description}
\end{description}

Since this holds for both directions, then we get the same harness of approximation factor for $\MOV^{\SPVF}$ too.
\end{proof}

%=============================================
%=============================================
